# Supplementary material for: Benchmark Design and Prior-independent Optimization
Source: arXiv:2001.10157 source file (2020-09-08)
Supplement: Supplementary file 1 [file aleck_notes.tex]

\section{Aleck Working Notes}

\subsection{Price Functions to Make an Adversary Indifferent}

\subsubsection{``Anonymous Truncation" Attempt at Prior Independent Price Setting Algorithm}
\textit{``Loosely" Towards Optimal Prior Independent Auctions} (2-agents, revenue).

\textbf{Prologue Discussion:}  The interest here was to try to use an intuitive setting and see if a mechanism could be designed to make an adversary indifferent over its full choice set, with respect to a multiplicative-approximation worst-case benchmark.  The result is less than desired, but the technique could very possibly be applied to a more interesting setting.

\begin{lemma}
The optimal prior independent auction will be:
\begin{enumerate}
    \item scale invariant,
    \item and a lookahead auction.
\end{enumerate}
\end{lemma}

\noindent \textbf{Intuition:}
\begin{enumerate}
    \item For purposes of analysis, fix $v_{\{2\}}$=1;
    \item triangle revenue curves are critical;
\begin{itemize}
    \item these are top-truncated at $\tau$, down-shifted EQRs (which are in the $\argmax$ set of the adversary);
    \item they have $\text{pdf}_k(x)=\frac{k}{(x+k)^2}$ on $\left[0,\tau\right]$ and a point mass at $\tau$ with weight $\frac{k}{\tau+k}$.
\end{itemize}
\end{enumerate}

\noindent \textbf{Idea:}
\begin{enumerate}
    \item fix class of triangle revenue curves with $k=1$, and let the truncation range over $\tau\geq 1$;
    \item fix $v_{\{2\}}=1$;
    \item adversary picks worst case $\tau\geq 1$
    \item (3) implies the algorithm designs a random pricing auction to agent $\{1\}$ to make adversary indifferent over all $\tau\geq 1$ (i.e., a distribution over rays coming out of origin on the revenue curve).
\end{enumerate}

\noindent \textbf{Notes:}
\begin{itemize}
    \item peak revenue for a triangle distribution with peak at $q$ and truncated at $\tau$ is $\tau\cdot q=(1-q)\cdot 1$ (from setting $k=1$);
    \item 2-agent opt revenue is $\tau\cdot q(2-q)=\frac{2\tau^2+\tau}{(\tau+1)^2}$, from:
\begin{align*}
    \tau(q) &= \frac{1-q}{q}\\
    q(\tau) &= \frac{1}{\tau+1}
\intertext{and}
    \text{opt-rev}(\tau,q) &= \tau(1-(1-q)^2)\\
    &= \tau(1-(1-2q+q^2))\\
    &= \tau\cdot q (2-q)
\end{align*}
\end{itemize}

\begin{lemma}
The algorithm must put a point mass on price $1=v_{\{2\}}$.
\end{lemma}

\noindent Algorithm chooses:
\begin{itemize}
    \item $\beta\in \left[0,1\right]$ as the point mass on 1;
    \item density function $f(t):[1,\infty)\rightarrow \mathbb{R}$, i.e., $f(t)\geq 0$ and $\int_1^{\infty}f(t)dt=1$.
\end{itemize}
\noindent to have
\begin{align*}
    \frac{\beta\cdot1 + (1-\beta)\int_1^{\tau}f(t)\cdot\text{price}(t)\cdot q(t)dt}{\tau\cdot q(2-q)}&=\alpha =\beta\cdot \gamma&
\intertext{for $\text{price}(t) = t$, $q(t) = 1/(t+1)$, and approximation ratio $\alpha$}
\Leftrightarrow &&\\
\intertext{(substitute out $q$ using $\tau(q)$, multiply through by the LHS denominator and divide by $\beta$)}
1+\frac{1-\beta}{\beta}\int_1^{\tau}f(t)\frac{t}{t+1}dt &= \gamma\cdot\frac{2\tau^2+\tau}{(1+\tau)^2}&
\end{align*}

\noindent \textbf{Technique:}
\begin{enumerate}
\item reduce the choice of $f(t)$ to choice of $g(t)$ such that $f(t)=\frac{\beta}{1-\beta}\cdot\gamma\cdot  g(t)$; this simplifies the needed equality to
\begin{equation*}
1+\gamma\cdot\int_1^{\tau}g(t)\frac{t}{t+1}dt = \gamma\cdot\frac{2\tau^2+\tau}{(1+\tau)^2}
\end{equation*}
where the $\frac{\beta}{1-\beta}$ term within $f(.)$ is particularly convenient because we need $f$ to be a density function and can now unilaterally use the parameter $\beta$ to re-normalize the density for any $\gamma$ and function $g$ with ``density converging" to non-infinity any constant.
\item Lower and upper integral end points need to cancel against the $(+1)$ additive term and the RHS, respectively:
\begin{itemize}
    \item the ``function form" of the RHS ignores multiplicative factors and is $\frac{2\tau^2+\tau}{(1+\tau)^2}$;
    \item upper end point matches the functional form of the RHS, which only happens if the integral evaluates to the functional form of the RHS;
    \item lower end points cancels the $(+1)$, with integral evaluating to the functional form, we can evaluate the integral at the lower end point and find it to be $\frac{2(1)^2+1}{(1+1)^2}=3/4$, to cancel the $(+1)$, this identifies $\gamma=4/3$ (note, a ``correct" should find obviated $\gamma =1$.
    \item We can take the derivative of the RHS functional form as a function of $t$ to find the functional form of the integrand $g(t)\frac{t}{t+1}$, and hence $g(t)$:
\begin{align*}
    \text{RHS}(t) &= \frac{2t^2+t}{(1+t)^2}\\
    \text{RHS}'(t) &= \frac{(t+1)^2(4t+1)-(2t^2+t)2(t+1)}{(t+1)^4}\\
    &= \frac{4t^2+t+4t+1-4t^2-2t}{(t+1)^3}=\frac{3t+1}{(t+1)^3}\\
    \text{RHS}'(t) &= g(t)\frac{t}{t+1}\\
    g(t) &= \frac{3t+1}{t(t+1)^2}
\end{align*}
\end{itemize}
\item The function $f(t)$ is a probability distribution depending on parameters $\beta, \gamma$ and our choice of $g(.)$; with $\gamma$ and $g(.)$ determined, we can identify $\beta$:
\begin{align*}
    f(t) &= \frac{\beta}{1-\beta}\cdot\gamma\cdot g(t)\\
    &= \frac{\beta}{1-\beta}\cdot\frac{4}{3}\cdot\frac{3t+1}{t(t+1)^2}\\
    \int_1^{\infty}f(t)dt &= 1\\
    \int_1^{\infty}\frac{\beta}{1-\beta}\cdot\frac{4}{3}\cdot\frac{3t+1}{t(t+1)^2}dt &= 1\\
    G(t) = \int\frac{3t+1}{t(t+1)^2}dt &= \frac{-2}{t+1}+\ln\left(\frac{t}{t+1}\right)\\
    \int_1^{\infty}g(t)dt=\left[\frac{-2}{t+1}+\ln\left(\frac{t}{t+1}\right)\right]_1^{\infty}&=1+\ln 2
\intertext{so}
    \frac{\beta}{1-\beta}\cdot\frac{4}{3}\cdot\left[1+\ln 2\right] &= 1\\
    \frac{\beta}{1-\beta}&= \frac{3}{4}\cdot\frac{1}{1+\ln 2}\\
    \beta&= \frac{3}{4}\cdot\frac{1}{1+\ln 2}(1-\beta)\\
    \beta&= \frac{3/4/(1+\ln 2)}{1+3/4/(1+\ln 2)}\approx .307
\intertext{and to summarize:}
\gamma = 4/3,~ \beta \approx .307,~ \alpha = \beta\cdot\gamma &\approx .409
\end{align*}
\end{enumerate}

\noindent \textbf{Final Technical Point:} relating to the lemma immediately following, our algorithm observes $\beta < alpha$ (equivalently $\gamma > 1$) because the benchmark is a bit odd.  The optimal revenue is set based on the possibility that both agents are drawn smaller than the truncation point including all values from the described distributions down to 0 ... even though we also have the assumption that $v_{\{2\}} =1$ which is technically inconsistent (though we can design the benchmark however we like for an ``arbitrary" game setting and analysis).

\begin{lemma}
The optimal prior independent mechanism must run the SPA with probability equal to its approximation factor, i.e., $\alpha =\beta$ for $\beta$ defined as above.
\end{lemma}

\newpage

\subsubsection{Fixed $q$, Adversary Indifferent over $\tau$}

\noindent \textbf{Starting Observations:}
\begin{itemize}
    \item peak revenue of a triangle revenue curve with peak at $q$ in quantile space and truncation $\tau$ in value space is $\tau q$
    \item the algorithm uses a randomized \textit{scale invariant} pricing function $\pi_{\text{inv}}$, putting $\alpha$ probability on $v_{\{2\}}$ and with probability $1-\alpha$ drawing from a continuous distribution with support $\left[v_{\{2\}},\infty\right)$
    \item the adversary gets the optimal revenue from 2 agents, which is $\tau q (2-q)$
    \item we use $dz$ to integrate in quantile space and $dy$ to integrate in price space (value space)
    \item given revenue curve straight line with slope $(-k) = \left( \frac{\tau q}{1-q}\right)$:
    \begin{itemize}
        \item height of curve at quantile $z$ is $(1-z)\left(\frac{\tau q}{1-q}\right)$
        \item inducing value $v(z) = \frac{1-z}{z}\frac{q}{1-q}\tau$
        \item from geometric identity, the quantile of a value (or price) is $q(y) = \frac{\frac{\tau q}{1-q}}{\frac{\tau q}{1-q}+y}=\frac{\tau q}{\tau q+(1-q)y}$
    \end{itemize}
    \item the density function for $q_{\{2\}}$ the larger of 2 random quantile draws from $U[0,1]$ (representing the weakly smaller value) is $q_{\{2\}}(x) = 2x$ on $[0,1]$
\end{itemize}

\noindent \textbf{The algorithm gets revenue from 3 pieces:}
\begin{enumerate}
    \item $\alpha \tau q^2+(1-\alpha)\cdot0$ when $v_{\{2\}}=\tau =v_{\{1\}}$
    \item $\alpha \int_q^1 \left[ \tau \frac{1-z}{z}\frac{q}{1-a}\right]\left(2zdz\right)=\left(\alpha \tau\frac{q}{1-q}\right)\left[2z-z^2\right]_q^1=\alpha \tau \frac{q}{1-q}\left[(1)-(2q-q^2)\right]=\alpha \tau q(1-q)$ when $v_{\{2\}}<\tau$ and posts price $v_{\{2\}}$
    \item $(1-\alpha)\int_q^1\int_{v(z)}^{\tau}(y)\left[\frac{\frac{\tau q}{1-q}}{\frac{\tau q}{1-q}+y}\left(\frac{1}{z}\right)\right]\left(\pi_{\text{inv}}(y,v(z))dy\right)2zdz$ when $v_{\{2\}}<\tau$ and the random price $y\sim \pi_{\text{inv}} > v_{\{2\}}$, where
    \begin{itemize}
        \item the outer integral ranges over $[q,1]$ the possible draws of $q_{\{2\}}$, and the inner integral ranges over $[v(z),\tau]$ the range of continuous random prices offered to $\{1\}$ \textit{which might sell} (prices above $\tau$ never sell)
        \item $(y)$ is the price conditioned on selling to $v_{\{1\}}$
        \item $\left[\frac{\frac{\tau q}{1-q}}{\frac{\tau q}{1-q}+y}\left(\frac{1}{z}\right)\right]$ is the probability of selling to agent $\{1\}$ given $v_{\{1\}}\geq v_{\{2\}}$
        \item $\left(\pi_{\text{inv}}(y,v(z))dy\right)$ is the density on price $y$ parameterized to be scale invariant by $v(z)$, and
        \item $2zdz$ is the density of $q_{\{2\}}$ at $z$
    \end{itemize}
\end{enumerate}
Following this, we also have
\begin{equation*}
    (1) + (2) = \alpha\left( \tau q^2 + \tau q (1-q)\right)=\alpha(\tau q)
\end{equation*}
The algorithm needs to choose $\pi_{\text{inv}}$ to satisfy the approximation ratio with equality as $\alpha = \frac{(1)+(2)+(3)}{\alpha \tau (2-q)}$:
\begin{align}
\label{eqn:approxformula}
    \alpha &= \frac{\alpha \tau q + (1-\alpha)\int_q^1\int_{v(z)}^{\tau}(y)\left[\frac{\tau q}{\tau q+(1-q)y}\right]\left(\pi_{\text{inv}}(y,v(z))dy\right)2dz }{\tau q (2-q)}
    \intertext{(cancel $\tau q$ RHS; multiply through by $(2-q)$; divide by $\alpha$; subtract 1)}
    (1-q) &= \left[2\cdot\frac{1-\alpha}{\alpha}\right]\int_q^1\int_{v(z)}^{\tau}\frac{y}{\tau q + (1-q)y}\cdot \pi_{\text{inv}}(y,v(z))dydz
\intertext{\textbf{Guess and calculate:} non-$v_{\{2\}}$ pricing density function $\pi_{\text{inv}}(y,v(z)) = \frac{v(z)}{y^2}$ on $\left[v(z),\infty\right)$.}
    (1-q) &=\left[2\cdot\frac{1-\alpha}{\alpha}\right]\int_q^1\left(v(z)\cdot \int_{v(z)}^{\tau}\frac{y}{\tau q + (1-q)y}\cdot\frac{1}{y^2}dy\right)dz
\intertext{(sub-calculation)}
\int_{v(z)}^{\tau}\frac{1}{y(\tau q + (1-q)y)}dy &= \left[\frac{1}{\tau q}\cdot \ln \left( \frac{y}{\tau q + (1-q)y}\right)\right]_{v(z)}^{\tau}\\
&= \left[ 0-\frac{1}{\tau q}\cdot\ln\left(\frac{v(z)}{\tau q + (1-q)v(z)}\right)\right]\\
&= \frac{-1}{\tau q}\cdot\ln\left( \frac{\frac{1-z}{z}\cdot\frac{q}{1-q}\tau}{\tau q+\frac{1-z}{z}q\tau}\right) = \frac{-1}{\tau q}\cdot\ln\left(\frac{1-z}{1-q}\right) > 0
\intertext{(where the evaluation greater than 0 is simply a sanity check)}
(1-q) &= \left[2\cdot\frac{1-\alpha}{\alpha}\right]\int_q^1\left(\frac{1-z}{z}\right)\left(\frac{q}{1-q}\right)\tau\cdot\frac{-1}{\tau q}\cdot \ln \left(\frac{1-z}{1-q}\right)dz\\
&= \left[2\cdot\frac{1-\alpha}{\alpha}\right]\left(\frac{1}{1-q}\right)\left[-\text{Li}_2(1-z)+(z-\ln z-1)\ln\left(\frac{1-z}{1-q}\right)-z \right]_q^1\\
&= \left[2\cdot\frac{1-\alpha}{\alpha}\right]\left(\frac{1}{1-q}\right)\left[(-0+0-1)-(-\text{Li}_2(1-q)+0-q) \right]\\
&= \left[2\cdot\frac{1-\alpha}{\alpha}\right]\left(\frac{1}{1-q}\right)\left[\sum_{k=1}^{\infty}\frac{(1-q)^k}{k^2}-(1-q)\right]\\
1 &= \left[2\cdot\frac{1-\alpha}{\alpha}\right]\cdot \sum_{k=2}^{\infty}\frac{(1-q)^{k-2}}{k^2}
\end{align}

\noindent where $\text{Li}_s(x)=\sum_{k=1}^{\infty}\frac{x^k}{k^s}$ is the polylogarithm function, here with parameter $s=2$; and which shows that if the algorithm picks $\alpha$, the adversary can pick a worst $q$; and if the algorithm knows a $q$ fixed in advance it can solve for $\alpha$ to make the adversary indifferent over all choices of $\tau$.

\newpage

\noindent\textbf{Guess and (partially) calculate:} non-$v_{\{2\}}$ pricing density function $\pi_{\text{inv}}(y,v(z)) = \frac{2\cdot(v(z))^2}{y^3}$ on $\left[v_{\{2\}},\infty\right)$.

\begin{align*}
    (1-q) &=\left[2\cdot\frac{1-\alpha}{\alpha}\right]\int_q^12\left(\left(v(z)\right)^2\cdot \int_{v(z)}^{\tau}\frac{y}{\tau q + (1-q)y}\cdot\frac{1}{y^3}dy\right)dz\\
    &= \left[2\cdot\frac{1-\alpha}{\alpha}\right]\int_q^12\left(\left(v(z)\right)^2\cdot \int_{v(z)}^{\tau}\frac{y}{\tau q + (1-q)y}\cdot\frac{1}{y^3}dy\right)dz
\intertext{(sub-calculation)}
\int_{v(z)}^{\tau}\frac{1}{y^2(\tau q+(1-q)y)}dy&=\left[ \frac{-1}{\tau qy}+\frac{1-q}{(\tau q)^2}\ln \left( \frac{\tau q+(1-q)y}{y}\right)\right]_{v(z)}^{\tau}\\
&= \left[\left(\frac{-q}{\tau^2q^2}+0\right)-\left(\left(\frac{z}{1-z}\right)\left(\frac{(-1)(1-q)}{\tau^2q^2}\right)+\frac{1-q}{(\tau q)^2}\ln\left(\frac{1+\frac{1-z}{z}}{\frac{1-z}{z}\cdot\frac{1}{1-q}}\right)\right)\right]\\
&= \left[\frac{(1-z)(-q)+z(1-q)}{\tau^2q^2(1-z)}-\frac{1-q}{\tau^2q^2}\ln\left(\frac{1-q}{1-z}\right) \right]\\
&= \frac{z-q}{\tau^2q^2(1-z)}-\frac{1-q}{\tau^2q^2}\ln\left(\frac{1-q}{1-z}\right)\\
(1-q) &= \left[4\frac{1-\alpha}{\alpha}\right]\int_q^1\left(\frac{(1-z)^2}{z^2}\cdot\frac{1}{(1-q)^2}\right)\left[ \frac{z-q}{1-z}-(1-q)\ln\left(\frac{1-q}{1-z}\right)\right]dz
\intertext{(which is also observed to be independent of $\tau$)}
\end{align*}

\noindent
\textbf{Attempts that did not make the problem easier:}
\begin{itemize}
    \item switching the order of integration, specifically from the ``\textbf{Guess and calculate}" lines; the region of integration is nice and the integral endpoints are still intuitive after switching the order, but it did not make the math easier, I was hoping for a solution that would isolate the power parameter;
    \item putting the exponential distribution (with arbitrary hazard rate) in as the scale-invariant pricing function;
\end{itemize}

\subsubsection{``Sub-Game" Analysis}

\textbf{What if approximation is not equal to the pricing function's point mass on $v_{\{2\}}$?}

In this subsection, we analyze the revenue of the auction under relaxation of the assumption that final prior independent approximation $\alpha$ is equal to the point mass probability $\beta$ which the optimal pricing function puts on $v_{\{2\}}$.

\begin{align}
\intertext{Starting from~\eqref{eqn:approxformula}}
     \alpha &= \frac{\alpha \tau q + (1-\alpha)\int_q^1\int_{v(z)}^{\tau}(y)\left[\frac{\tau q}{\tau q+(1-q)y}\right]\left(\pi_{\text{inv}}(y,v(z))dy\right)2dz }{\tau q (2-q)}
    \intertext{(breaking equality, $\alpha$ on the RHS is replaced with $\beta$)}
     \alpha &= \frac{\beta + (1-\beta)\int_q^1\int_{v(z)}^{\tau}(y)\left[\frac{1}{\tau q+(1-q)y}\right]\left(\pi_{\text{inv}}(y,v(z))dy\right)2dz }{(2-q)}
    \intertext{(similar to above)~~\textbf{Guess and calculate:} non-$v_{\{2\}}$ pricing density function $\pi_{\text{inv}}(y,v(z)) = \frac{v(z)}{y^2}$ on $\left[v(z),\infty\right)$.}
     \alpha &= \frac{\beta + 2(1-\beta)\int_q^1\int_{v(z)}^{\tau}\left[\frac{y}{\tau q+(1-q)y}\right]\cdot \frac{v(z)}{y^2} dy dz }{(2-q)}\\
    \alpha &= \frac{\beta + 2(1-\beta)\int_q^1\left(\frac{1-z}{z} \right)\frac{\tau q}{1-q}\cdot \int_{v(z)}^{\tau}\left[\frac{1}{y(\tau q+(1-q)y)}\right] dy dz }{(2-q)}\\
    \alpha &= \frac{\beta + 2(1-\beta)\int_q^1\left(\frac{1-z}{z} \right)\frac{\tau q}{1-q}\cdot \frac{-1}{\tau q}\ln \left( \frac{1-z}{1-q}\right) dz }{(2-q)}\\
\intertext{and for the next step, the last integral was resolved in more detail above (where it was assumed $\alpha = \beta$}
\label{eqn:alphabeta}
    \alpha &= \frac{\beta + 2(1-\beta)\left[\sum_{k=2}^{\infty} \frac{(1-q)^{k-1}}{k^2} \right] }{(2-q)}
\end{align}

\noindent\textit{we repeat the preceding calculation for the cubic density function}

\begin{align}
\intertext{Starting from scratch for cubic pricing:}
     &\alpha = \frac{\alpha \tau q + (1-\alpha)\int_q^1\int_{v(z)}^{\tau}(y)\left[\frac{\tau q}{\tau q+(1-q)y}\right]\left(\pi_{\text{inv}}(y,v(z))dy\right)2dz }{\tau q (2-q)}
    \intertext{(breaking equality, $\alpha$ on the RHS is replaced with $\beta$)}
     &= \frac{\beta + (1-\beta)\int_q^1\int_{v(z)}^{\tau}(y)\left[\frac{1}{\tau q+(1-q)y}\right]\left(\pi_{\text{inv}}(y,v(z))dy\right)2dz }{(2-q)}
    \intertext{(similar to above)~~\textbf{Guess and calculate:} non-$v_{\{2\}}$ pricing density function $\pi_{\text{inv}}(y,v(z)) = \frac{2(v(z))^2}{y^3}$ on $\left[v(z),\infty\right)$.}
    &= \frac{\beta + 2(1-\beta)\int_q^1\int_{v(z)}^{\tau}(y)\left[\frac{1}{\tau q+(1-q)y}\right]\left(\frac{2(v(z))^2}{y^3}\right)dydz }{(2-q)}\\
    &= \frac{\beta + 4(1-\beta)\int_q^1\left(\frac{1-z}{z} \right)^2\left(\frac{\tau q}{1-q}\right)^2\cdot \int_{v(z)}^{\tau}\left[\frac{1}{y(\tau q+(1-q)y)}\right] dy dz }{(2-q)}\\
    &= \frac{\beta + 4(1-\beta)\int_q^1\left(\frac{1-z}{z} \right)^2\left(\frac{\tau q}{1-q}\right)^2\cdot \left[\frac{z-q}{\tau^2 q^2(1-z)}+\frac{-(1-q)}{\tau^2 q^2}\ln \left( \frac{1-z}{1-q}\right) \right]dz }{(2-q)}\\
\label{eqn:int3needsderiv}
    &= \frac{\beta + \frac{4(1-\beta)}{(1-q)^2}\int_q^1\left(\frac{1-z}{z} \right)^2\cdot \left[\frac{z-q}{(1-z)}-(1-q)\ln \left( \frac{1-z}{1-q}\right) \right]dz }{(2-q)}
\intertext{The next calculation  of the integral was by WolframAlpha.  We give some notes for repeating the calculation.  It gives one additive term as $-(q-1)\ln(z-1)$, which we replaced by $+(1-q)\ln(1-z)$, which is clearly the form we want to use.  These two components are interchangeable because they have the same derivative.  Further, six of the output terms need to combine `$1$' and `$-q$' terms into `$1-q$' terms, and additional simplification from there is needed to arrive at the anti-derivative function that we give (with the $+(1-q)\ln(1-z)$ merging with other terms in these last steps).  We confirm this is indeed the anti-derivative function by calculating its derivative and confirming the function inside of the integral in line~\eqref{eqn:int3needsderiv} (calculation below)}
    &= \frac{\beta + \frac{4(1-\beta)}{(1-q)^2}\left[-2(1-q)\text{Li}_2(z)+\frac{q(1-z^2)}{z} +(1-q)\left(\frac{1}{z}-z \right)\ln\left(\frac{1-z}{1-q} \right)+2\ln z(1-(1-q)\ln(1-q))\right]_q^1}{(2-q)}
\intertext{(the next line uses the fact that $\lim_{z\rightarrow 1} (1/z-z)\cdot \ln (1-z) = 0$)}
    &= \frac{\beta + \frac{4(1-\beta)}{(1-q)^2}\left[\left(-2(1-q)\text{Li}_2(1)\right)-\left(-2(1-q)\text{Li}_2(q)+(1-q^2) +2\ln q(1-(1-q)\ln(1-q))\right)\right]}{(2-q)}\\
\intertext{(cancel a factor of $(1-q)$)}
    &= \frac{\beta + \frac{4(1-\beta)}{(1-q)}\left[-2\cdot \text{Li}_2(1)+2\cdot \text{Li}_2(q)-(1+q) -\frac{2}{1-q}\ln(1-(1-q)) +2\ln q\ln(1-q) \right]}{(2-q)}\\
\intertext{(substitute in the Taylor series for $\ln$ and $\text{Li}_2$)}
    &= \frac{\beta + \frac{4(1-\beta)}{(1-q)}\left[-2\cdot \sum_{k=1}^{\infty}\frac{1}{k^2}+2\cdot \sum_{k=1}^{\infty}\frac{q^k}{k^2}-(1+q) +2\sum_{k=1}^{\infty}\frac{(1-q)^{k-1}}{k} +2\ln q\ln(1-q) \right]}{(2-q)}\\
\intertext{(combine the two $\text{Li}_2$ Taylor series; remove and combine the first term of the $\ln$ Taylor series)}
    &= \frac{\beta + \frac{4(1-\beta)}{(1-q)}\left[-2\cdot \sum_{k=1}^{\infty}\frac{1-q^k}{k^2}+(1-q) +2\sum_{k=2}^{\infty}\frac{(1-q)^{k-1}}{k} +2\ln (1-(1-q))\ln(1-q) \right]}{(2-q)}\\
\intertext{(factor $(1-q)$ out of the numerator of the first sum)}
    &= \frac{\beta + \frac{4(1-\beta)}{(1-q)}\left[-2\cdot \sum_{k=1}^{\infty}\frac{(1-q)\sum_{j=0}^{k-1}q^j}{k^2}+(1-q) +2\sum_{k=2}^{\infty}\frac{(1-q)^{k-1}}{k} +2\ln (1-(1-q))\ln(1-q) \right]}{(2-q)}\\
\intertext{(substitute in another $\ln$ Taylor series and cancel another factor of $(1-q)$)}
    &= \frac{\beta + 4(1-\beta)\left[-2\cdot \sum_{k=1}^{\infty}\frac{\sum_{j=0}^{k-1}q^j}{k^2}+1 +2\sum_{k=2}^{\infty}\frac{(1-q)^{k-2}}{k} -2\cdot\ln(1-q)\cdot \sum_{k=1}^{\infty}\frac{(1-q)^{k-1}}{k} \right]}{(2-q)}\\
    &= \frac{\beta + 4(1-\beta)\left[-2\cdot \sum_{k=2}^{\infty}\frac{\sum_{j=0}^{k-1}q^j}{k^2}-1-2\ln(1-q) +2\sum_{k=2}^{\infty}\frac{(1-q)^{k-2}}{k} -2\cdot\ln(1-q)\cdot \sum_{k=2}^{\infty}\frac{(1-q)^{k-1}}{k} \right]}{(2-q)}
\end{align}

\noindent For completeness, the derivative to prove the correct substitution into line~\eqref{eqn:int3needsderiv}:
\begin{align*}
    f(z)=& -2(1-q)\text{Li}_2(z)+\frac{q(1-z^2)}{z} +(1-q)\left(\frac{1}{z}-z \right)\ln\left(\frac{1-z}{1-q} \right)+2\ln z(1-(1-q)\ln(1-q))\\
    =& -2(1-q)\text{Li}_2(z)-qz+\frac{q}{z}+2\ln z - (1-q)z\ln\left(\frac{1-z}{1-q}\right)+(1-q)\frac{1}{z}\ln\left(\frac{1-z}{1-q}\right)\\
    &-(1-q)\ln(1-q)\cdot 2\cdot \ln z\\
    f'(z) =& 2(1-q)\frac{\ln(1-z)}{z}-q-\frac{q}{z^2}+\frac{2}{z}-(1-q)\ln \left(\frac{1-z}{1-q}\right)+\frac{(1-q)z}{(1-z)}\\
    &+(1-q)\frac{-1}{z^2}\left(\frac{1-z}{1-q}\right)+(1-q)\frac{1}{z}\cdot\frac{-1}{(1-z)}-(1-q)\ln(1-q)\cdot2\cdot\frac{1}{z}\\
    =& \left[2(1-q)\frac{\ln(1-z)}{z}-(1-q)\ln(1-q)\cdot2\cdot\frac{1}{z}-(1-q)\ln \left(\frac{1-z}{1-q}\right)+(1-q)\frac{-1}{z^2}\left(\frac{1-z}{1-q}\right)\right]\\
    &+\left[-q-\frac{q}{z^2}+\frac{2}{z}+\frac{(1-q)z}{(1-z)}+(1-q)\frac{1}{z}\cdot\frac{-1}{(1-z)}\right]\\
    =& \left[\frac{2z(1-q)}{z^2}\ln\left(\frac{1-z}{1-q}\right)-\frac{z^2(1-q)}{z^2}\ln\left(\frac{1-z}{1-q}\right)-\frac{(1-q)}{z^2}\ln\left(\frac{1-z}{1-q}\right) \right]\\
    &+ \left[\frac{-qz^2(1-z)-q(1-z)+2z(1-z)+(1-q)z^3-(1-q)z}{z^2(1-z)} \right]\\
    =& \left[\frac{-(1-z)^2}{z^2}(1-q)\ln\left(\frac{1-z}{1-q}\right)\right]+ \left[\frac{-qz^2+qz^3-q+qz+2z-2z^2+z^3-qz^3-z+qz}{z^2(1-z)} \right]\\
    =& \left[\frac{-(1-z)^2}{z^2}(1-q)\ln\left(\frac{1-z}{1-q}\right)\right]+ \left[\frac{qz(1-z)-z^2(1-z)+z(1-z)-q(1-z)}{z^2(1-z)}\right]\\
    =& \left[\frac{-(1-z)^2}{z^2}(1-q)\ln\left(\frac{1-z}{1-q}\right)\right]+ \left[\frac{(1-z)(z-q)}{z^2}\right]\\
    =& \left[\frac{-(1-z)^2}{z^2}(1-q)\ln\left(\frac{1-z}{1-q}\right)\right]+ \left[\frac{(1-z)^2}{z^2}\cdot\frac{z-q}{1-z}\right]~~\checkmark
\end{align*}

\begin{prop}
For {\em quadratic pricing}.  By numerically searching $\beta\in [0.5, 1]$ and $q\in [0,1]$, we can try to solve $\max_{\beta} min_{q}~\alpha$ as the approximation ratio given the choice of the algorithm to put $(1-\beta)$ weight on quadratic pricing and the rest $\beta$ weight as a point mass on $v_{\{2\}}$.
\end{prop}
\noindent \textbf{Claim:} The optimal approximation of quadratic pricing uses $\beta \approx 0.8435$ and results in $\alpha\approx 0.5154$.  This claim should be re-checked independently.

Next we take two derivatives of line~\eqref{eqn:alphabeta} with respect to $q$, and show that the result is positive, therefore after fixing $\beta$, approximation is convex in $q$.  I.e., this shows that the $\argmin$-solution to the inner program of $\left[\max_{\beta} min_{q}~\alpha\right]$ can be found using binary search.  We define a new function $A_{\text{quad}}(\beta,q)$ to be the approximation ratio given quadratic pricing function mixed with the point mass on $v_{\{2\}}$, treating $\beta$ and $q$ as variables.

\begin{align}
    A_{\text{quad}} &= \frac{\beta + 2(1-\beta)\left[\sum_{k=2}^{\infty} \frac{(1-q)^{k-1}}{k^2} \right] }{(2-q)}\\
    \frac{\partial A'_{\text{quad}}}{\partial q} &=  \frac{(2-q)\cdot\left( 2(1-\beta)\left[\sum_{k=2}^{\infty}\frac{(k-1)(1-q)^{k-2}\cdot (-1)}{k^2} \right]\right) -\left(\beta + 2(1-\beta)\left[\sum_{k=2}^{\infty} \frac{(1-q)^{k-1}}{k^2} \right]\right)\cdot (-1) }{(2-q)^2}\\
    %\frac{\partial A'_{\text{quad}}}{\partial q}
    &=  \frac{\beta+\left( 2(1-\beta)\left[\sum_{k=2}^{\infty}\frac{(1-q)^{k-1}-(k-1)(2-q)(1-q)^{k-2}}{k^2} \right]\right) }{(2-q)^2}\\
    &= \frac{\beta+\left( 2(1-\beta)\left[\sum_{k=2}^{\infty}\frac{(3-2q-k(2-q))\cdot (1-q)^{k-2}}{k^2} \right]\right) }{(2-q)^2}\\
    &= \frac{\beta+\left( 2(1-\beta)\left[\frac{-1}{4}+\sum_{k=3}^{\infty}\frac{(3-2q-k(2-q))\cdot (1-q)^{k-2}}{k^2} \right]\right) }{(2-q)^2}\\
    &= \frac{(\frac{-1}{2}+\frac{3}{2}\beta)}{(2-q)^2}+\frac{\left( 2(1-\beta)\left[\sum_{k=3}^{\infty}\frac{(3-2q-k(2-q))\cdot (1-q)^{k-2}}{k^2} \right]\right) }{(2-q)^2}
\end{align}
\begin{align}
    \frac{\partial A''_{\text{quad}}}{\partial q} &=
    \frac{(-1+3\beta)}{(2-q)^3}+\frac{\left( 4(1-\beta)\left[\sum_{k=3}^{\infty}\frac{(3-2q-k(2-q))\cdot (1-q)^{k-2}}{k^2} \right]\right) }{(2-q)^3}\\
    &+\frac{(2-q)\left( 2(1-\beta)\left[\sum_{k=3}^{\infty}\frac{(3-2q-k(2-q))\cdot (1-q)^{k-3}\cdot(k-2)(-1)+(k-2)\cdot (1-q)^{k-2}}{k^2} \right]\right) }{(2-q)^3}\\
    &=
    \frac{(-1+3\beta)}{(2-q)^3}+\frac{\left( 4(1-\beta)\left[\sum_{k=3}^{\infty}\frac{(3-2q-k(2-q))\cdot (1-q)(1-q)^{k-3}}{k^2} \right]\right) }{(2-q)^3}\\
    &+\frac{(2-q)\left( 2(1-\beta)\left[\sum_{k=3}^{\infty}\frac{(3-2q-k(2-q))\cdot (1-q)^{k-3}\cdot(k-2)(-1)+(k-2)\cdot (1-q)(1-q)^{k-3}}{k^2} \right]\right) }{(2-q)^3}\\
    &=
    \frac{(-1+3\beta)}{(2-q)^3}+\frac{\left( 4(1-\beta)\left[\sum_{k=3}^{\infty}\frac{(3-2q-k(2-q))\cdot (1-q)(1-q)^{k-3}}{k^2} \right]\right) }{(2-q)^3}\\
    &+\frac{(2-q)\left( 2(1-\beta)\left[\sum_{k=3}^{\infty}\frac{(k-1)(2-q)(k-2)(1-q)^{k-3}}{k^2} \right]\right) }{(2-q)^3}\\
    &=
    \frac{(-1+3\beta)}{(2-q)^3}+\frac{\left( 4(1-\beta)\left[\frac{(-3+q)(1-q)}{9}+\sum_{k=4}^{\infty}\frac{(3-2q-k(2-q))\cdot (1-q)(1-q)^{k-3}}{k^2} \right]\right) }{(2-q)^3}\\
    &+\frac{(2-q)\left( 2(1-\beta)\left[\frac{2-q}{9}+\sum_{k=4}^{\infty}\frac{(k-1)(2-q)(k-2)(1-q)^{k-3}}{k^2} \right]\right) }{(2-q)^3}\\
    &=
    \frac{(-1+3\beta)}{(2-q)^3}+\frac{\frac{(1-\beta)}{9}\cdot4\cdot(-3+q)(1-q)+\left( 4(1-\beta)\left[\sum_{k=4}^{\infty}\frac{(3-2q-k(2-q))\cdot (1-q)(1-q)^{k-3}}{k^2} \right]\right) }{(2-q)^3}\\
    &+\frac{\frac{(1-\beta)}{9}\cdot2\cdot(2-q)(2-q)+(2-q)\left( 2(1-\beta)\left[\sum_{k=4}^{\infty}\frac{(k-1)(2-q)(k-2)(1-q)^{k-3}}{k^2} \right]\right) }{(2-q)^3}\\
    &=
    \left[\frac{(-1+3\beta)}{(2-q)^3}+\frac{\frac{(1-\beta)}{9}\left(-4+2q(1-q) \right)}{(2-q)^3}\right]+\frac{\left( 4(1-\beta)\left[\sum_{k=4}^{\infty}\frac{(3-2q-k(2-q))\cdot (1-q)(1-q)^{k-3}}{k^2} \right]\right) }{(2-q)^3}\\
    &+\frac{(2-q)\left( 2(1-\beta)\left[\sum_{k=4}^{\infty}\frac{(k-1)(2-q)(k-2)(1-q)^{k-3}}{k^2} \right]\right) }{(2-q)^3}
\intertext{(and within the first brackets, by $\beta\in [ 1/2,1]$ and $q\in[0,1]$, the first numerator is at least 1/2, and the second has magnitude less than 1/2)}
    &>
    \frac{\left( 4(1-\beta)\left[\sum_{k=4}^{\infty}\frac{(3-2q-k(2-q))\cdot (1-q)(1-q)^{k-3}}{k^2} \right]\right) }{(2-q)^3}\\
    &+\frac{(2-q)\left( 2(1-\beta)\left[\sum_{k=4}^{\infty}\frac{(k-1)(2-q)(k-2)(1-q)^{k-3}}{k^2} \right]\right) }{(2-q)^3}
\intertext{(and now that we have the sum for all $k\geq 4$, we can lower bound $(k-1)(k-2)$ by $k$ in the second term)}
    &\geq
    \frac{\left( 4(1-\beta)\left[\sum_{k=4}^{\infty}\frac{(3-2q-k(2-q))\cdot (1-q)(1-q)^{k-3}}{k^2} \right]\right) }{(2-q)^3}+\frac{(2-q)\left( 2(1-\beta)\left[\sum_{k=4}^{\infty}\frac{k(2-q)(1-q)^{k-3}}{k^2} \right]\right) }{(2-q)^3}
\intertext{(and now we can simplify because $2(2-q)\geq 4(1-q)$, resulting in a quantity in which all terms are positive.)}
    &\geq
    \frac{\left( 4(1-\beta)\left[\sum_{k=4}^{\infty}\frac{(3-2q)\cdot (1-q)(1-q)^{k-3}}{k^2} \right]\right) }{(2-q)^3}\geq 0 ~\checkmark
    %\intertext{(re-arrange the second and third terms into negative and positive terms)}
    %&=
    %\frac{(-1+3\beta)}{(2-q)^3}-\frac{\left( (1-\beta)\left[\sum_{k=3}^{\infty}\frac{\left[4k(2-q)\cdot (1-q)+(2-q)\cdot2\cdot(3-2q)(k-2)\right]\left[(1-q)^{k-3}\right]}{k^2} \right]\right) }{(2-q)^3}\\
    %&+\frac{\left( (1-\beta)\left[\sum_{k=3}^{\infty}\frac{\left[4(3-2q)(1-q)+(2-q)\cdot2\cdot k(2-q)(k-2)+(2-q)\cdot2\cdot(k-2) (1-q)\right]\left[(1-q)^{k-3}\right]}{k^2} \right]\right) }{(2-q)^3}
\end{align}

\begin{lemma}
Point mass on $v_{\{2\}}$ is $\beta\geq \alpha$ the approximation ratio.
\end{lemma}
\begin{proof}
The pricing function gets $\beta$ approximation on point-mass distributions which are regular, establishing (this direction of the inequality.

As a note, equality is conjectured.
\end{proof}

\subsubsection{Definition of ``scale-invariant" pricing functions for lookahead auctions}

\begin{definition}
\label{def:scale}
A look-ahead auction's random {\em pricing function}- i.e., the function $\pi$ (as pdf) describing the random price offered to the agent with largest type- is {\em scale invariant} in the second highest value $\alpha=v_{\{2\}}$ if it satisfies
\begin{align*}
    \Pi_k(x) &= \Pi_{\alpha k}(\alpha x)\\
    \pi_k(x) &= \alpha\cdot \pi_{\alpha k}(\alpha x)
\end{align*}
\end{definition}

To add a little more detail here.  The idea is that we start with a (cdf) distribution $F(z)$ with support $z\in[1,\infty)$ and standard deviation 1.  Note that {\em standard deviation} and {\em scale} are actually equivalent.  We transform the distribution into $F_k(x)$ according to parameter $k$, which needs to be both the new standard deviation, and the new lower bound on support.

\begin{align}
    F_k(x) = F(\frac{x}{k})\\
    k\cdot f_k(x) = f(\frac{x}{k})
\end{align}

\noindent where it is now obvious that the multiplicative factor of $k$ is needed (generally) to cancel out the effects of chain rule upon taking the partial of $F$ with respect to $x$.

\subsubsection{Proof Attempt at Sufficiency of Triangle Revenue Curves for Adversary in response to Algorithm as Lookahead with Scale-Invariant Pricing Function}

\begin{definition}
Call an auction algorithm {\em unbiased} if it is a {\em lookahead auction with scale-invariant pricing function}, i.e., if it
\begin{itemize}
    \item only ever allocates the item to the agent with largest value $v_{\{1\}}$ (WLOG use agent 1 as the highest value);
    \item looks at all small values up to $v_{\{2\}}$ the second-highest value and then offers agent 1 a random price according to distribution $\pi_k$ with support a subset of $\left[v_{\{2\}},\right)\infty)$;
    \item the funcion $\pi_k$ is scale-invariant in its bound-on-lower-support parameter $k$ with $k=v_{\{2\}}$ for our purposes.
\end{itemize}
\end{definition}

\begin{prop}
Consider any {\em unbiased} auction algorithm \texttt{ALG}.  For the class of distributions characterized by a fixed peak revenue point $(q,R)$ in the ``revenue-curve plane," the prior independent adversary (restricted to the class of regular distributions, versus DSIC auctions) strictly prefers either the triangle revenue curve with peak $(q,R)$ or the point mass distribution at value $R/q$, in comparison to each other element of the class.strictly prefers the triangle revenue curve with peak $(q,R)$ over any other element of the class.
\end{prop}
\begin{proof}
We are going to prove the revenue inequality pointwise for every realized value of $q_{\{2\}}$, covering all $q_{\{2\}}$ by two cases.  These two cases break down naturally based on the realized (larger) quantile $q_{\{2\}}$ being below or above the fixed $q$ from the problem statement.  We can consider the cases separately because of independence of the analyses generally, and specifically by linearity of expectation.

First we will show that- holding the rest of the distribution fixed, the adversary strictly prefers to truncate the distribution at $\tau= R/q$, creating the ``left side" of the triangle as a line-segment from $(0,0)$ to the peak.  Second we will show that- again holding the behavior at truncation and now smaller quantiles fixed- the adversary strictly prefers the distribution below the truncation point (in value / price space) to be the constant-negative-virtual-value distribution (CNVV) with virtual value equal to $-R/(1-q)=-\tau q/(1-q)$, creating the ``right side" of the triangle as a line-segment from the peak to $(1,0)$.

For the first part, we give an analysis of the ratio of revenue performances between the optimal algorithms (knowing the regular distribution $\Gamma$ and the truncated (``half-triangle) distribution $\Delta$) and the unbaised algorithm \texttt{ALG}, for both distributions.  Let $P_{q^2}^F\geq 0, ~P_{1-q^2}^{F}\geq 0$ be the revenues that the algorithm gets when it posts its random price above $v_{\{2\}}$ versus distribution $F$ (i.e., the random price it draws is not realized as the point mass on $v_{\{2\}}$), respectively when both value draws are realized to have quantile smaller than $q$ (with probability $q^2$), and otherwise (with probability $1-q^2$).
\begin{align*}
\intertext{For the original arbitrary, fixed regular distribution $\Gamma$ (with peak at $(q,R)$):}
    &\frac{\texttt{OPT}_{\Gamma}}{\texttt{ALG}_{\Gamma}}
    = \frac{\left[\text{Rev}(\texttt{OPT}_{\Gamma})|q_{\{2\}}\leq q\right]+\left[\text{Rev}(\texttt{OPT}_{\Gamma})|q_{\{1\}}\leq q,~q_{\{2\}}\geq q\right]+\left[\text{Rev}(\texttt{OPT}_{\Gamma})|q_{\{1\}}> q\right]}{\left[\text{Rev}(\texttt{ALG}_{\Gamma})|q_{\{2\}}\leq q\right]+\left[\text{Rev}(\texttt{ALG}_{\Gamma})|q_{\{2\}}> q\right]}\\
    &=\frac{\left[q^2\mathbf{E}_{\Gamma}\left[v_{\{2\}}|v_{\{2\}}\geq \tau\right]\right]+\left[2q(1-q)\cdot \tau\right] +\left[(1-q)^2\cdot0\right]}{\left[q^2\left(\alpha\cdot\mathbf{E}_{\Gamma}\left[v_{\{2\}}|v_{\{2\}}\geq \tau\right]+P_{q^2}^{\Gamma}\right)\right]+\left[((1-q^2)\left(\alpha\cdot\mathbf{E}_{\Gamma}\left[v_{\{2\}}|v_{\{2\}}< \tau\right]+P_{1-q^2}^{\Gamma}\right)\right]}\\
\intertext{we re-arrange and conveneniently label quantities:}
&=\frac{\left[A'=q^2\mathbf{E}_{\Gamma}\left[v_{\{2\}}|v_{\{2\}}\geq \tau\right]\right]+\left[B'=2q(1-q)\cdot \tau\right]}{\left[A''=q^2\left(\alpha\cdot\mathbf{E}_{\Gamma}\left[v_{\{2\}}|v_{\{2\}}\geq \tau\right]\right)\right]+\left[B''=q^2\cdot P_{q^2}^{\Gamma}+((1-q^2)\left(\alpha\cdot\mathbf{E}_{\Gamma}\left[v_{\{2\}}|v_{\{2\}}< \tau\right]+P_{1-q^2}^{\Gamma}\right)\right]}\\
\intertext{and for the truncated half-triangle distribution $\Delta$:}
& \frac{\texttt{OPT}_{\Delta}}{\texttt{ALG}_{\Delta}} = \frac{\left[\text{Rev}(\texttt{OPT}_{\Delta})|q_{\{2\}}\leq q\right]+\left[\text{Rev}(\texttt{OPT}_{\Delta})|q_{\{1\}}\leq q,~q_{\{2\}}\geq q\right]+\left[\text{Rev}(\texttt{OPT}_{\Delta})|q_{\{1\}}> q\right]}{\left[\text{Rev}(\texttt{ALG}_{\Delta})|q_{\{2\}}\leq q\right]+\left[\text{Rev}(\texttt{ALG}_{\Delta})|q_{\{2\}}> q\right]}\\
&= \frac{\left[q^2\cdot\tau\right] + \left[2q(1-q)\tau\right]+\left[(1-q)^2\cdot 0\right]}{\left[\alpha q^2\cdot\tau\right]+\left[((1-q^2)\left(\alpha\cdot\mathbf{E}_{\Delta}\left[v_{\{2\}}|v_{\{2\}}< \tau\right]+P_{1-q^2}^{\Delta}\right)\right]}\\
\intertext{again adding some labels:}
&= \frac{\left[C'=q^2\cdot\tau\right] + \left[2q(1-q)\tau\right]}{\left[C''=\alpha q^2\cdot\tau\right]+\left[((1-q^2)\left(\alpha\cdot\mathbf{E}_{\Delta}\left[v_{\{2\}}|v_{\{2\}}< \tau\right]+P_{1-q^2}^{\Delta}\right)\right]}\\
\intertext{and we are interested in the ratios:}
& A=\frac{A'}{A''},~~ B=\frac{B'}{B''},~~C=\frac{C'}{C''}
\end{align*}

Note that after reducing, $A=C=1/\alpha$, though $A$ has numerator $A'$ and denominator $A''$ multiplied by the constant ``heavier weight," i.e., obviously the weight as [(second price) revenue conditioned on $v_{\{2\}}$ at least the Myerson price $\tau$] is at least the weight as [truncation value $\tau$].

Now we consider two cases as $A\geq B$ and $A\leq B$.  For the first case, notice that in fact $A=C=1/\alpha$ is the exact ratio that would be obtained by a point mass distribution at $\tau$, so when $A\geq B$ it follows that the ratio $\texttt{OPT}/\texttt{ALG}$ will be larger using the point mass distribution compared to using $F$.  For the second case, the ratio gets larger replacing $A', A''$ with $C',C''$ respectively- because as mentioned the multiplier is heavier in the $A$ ratio and the total ratio increases when $A\leq B$ and the ``weight" on $A$ decreases:
\begin{align*}
&\frac{\texttt{OPT}_{\Gamma}}{\texttt{ALG}_{\Gamma}}= \frac{\left[q^2\mathbf{E}_{\Gamma}\left[v_{\{2\}}|v_{\{2\}}\geq \tau\right]\right]+\left[2q(1-q)\cdot \tau\right] }{\left[q^2\left(\alpha\cdot\mathbf{E}_{\Gamma}\left[v_{\{2\}}|v_{\{2\}}\geq \tau\right]\right)\right]+\left[q^2\cdot P_{q^2}^{\Gamma}+((1-q^2)\left(\alpha\cdot\mathbf{E}_{\Gamma}\left[v_{\{2\}}|v_{\{2\}}< \tau\right]+P_{1-q^2}^{\Gamma}\right)\right]}\\
& \leq \frac{\left[q^2\cdot\tau\right]+\left[2q(1-q)\cdot \tau\right] }{\left[q^2\left(\alpha\cdot\tau\right)\right]+\left[q^2\cdot P_{q^2}^{\Gamma}+((1-q^2)\left(\alpha\cdot\mathbf{E}_{\Gamma}\left[v_{\{2\}}|v_{\{2\}}< \tau\right]+P_{1-q^2}^{\Gamma}\right)\right]}\\
&\leq \frac{\left[q^2\cdot\tau\right]+\left[2q(1-q)\cdot \tau\right] }{\left[q^2\left(\alpha\cdot\tau\right)\right]+\left[((1-q^2)\left(\alpha\cdot\mathbf{E}_{\Gamma}\left[v_{\{2\}}|v_{\{2\}}< \tau\right]+P_{1-q^2}^{\Delta}\right)\right]}=\frac{\texttt{OPT}_{\Delta}}{\texttt{ALG}_{\Delta}}
\end{align*}
with the other differences in terms handled trivially in the second inequality because the denominator can only get smaller by $P_{q^2}^{\Gamma}\geq 0$ and $P_{1-q^2}^{\Gamma}\geq P_{1-q^2}^{\Delta}$.

For the second sub-claim, we start by noting that we may restrict our attention to starting with the class of regular distributions which are truncated at the top, including all point masses and all regular distributions with peak revenue at $(q,R)$ for strictly $q<1$ which are truncated at $R/q$.  All other regular distributions have been excluded from consideration by the previous argument.

We also note that $\texttt{OPT}_{( \cdot )}$ has equal performance across all regular distribution shapes below the peak, because they all post the Myerson reserve price at the peak (uniquely identified by the proposed truncation value).  For the rest of the proof, the goal of the adversary is simply to ``design" the regular distribution pdf below the truncation value to minimize the performance of fixed \texttt{ALG}.

The argument for this second case continues by arguing that, for every realized (larger) quantile $q_{\{2\}}\in\left[q,1\right)$, performance of the algorithm would be smallest if the distribution is chosen as the CNVV making up the triangle distribution.  This is sufficient because it will hold pointwise for every such $q_{\{2\}}$.

Let the arbitrary regular distribution with peak at $(q,R)$ be labeled by $\delta$, and the triangle curve for comparison be labeled by $\gamma$.  In particular, for a fixed $q_{\{2\}}$, let $\delta$ be the value $v_{\delta}(q_{\{2}\})$, and let $\gamma$ be the value $v_{\gamma}(q_{\{2\}})$, i.e. the values associated with $q_{\{2\}}$ according to the respective revenue curves.

We observe that if the scale-invariant price function $\pi_k$ puts a point mass on $k$, then it will clearly get more revenue from the point mass probability when the buyer's revenue curve is the arbitrary $\delta$ curve rather than the $\gamma$ curve.  Now from this point on, %WLOG we can ignore a point mass on $k$ and consider $\pi_k$ to be a function with total measure 1 on prices strictly above $k$ (equivalently, 
WLOG condition otherwise on the randomly drawn price being above $k$ (recall that $k$ is the scale invariant parameter of the price function so it corresponds to both $\delta$ and $\gamma$ respectively).  This induces new revenue curves for a single agent 1, having conditioned on $q_{\{1\}}\leq q_{\{2\}}$.  We overload labeling and still use $\delta$ and $\gamma$ to refer to their respectively conditioned curves.  They new curves now both realize their peaks at quantile $q/q_{\{2\}}$, and have maximum revenue equal to $\tau\cdot q/q_{\{2\}}$.

We now lower bound the performance of the $\delta$-curve by the curve $\delta'$ which irons $\delta$ between $q/q_{\{2\}}$ and 1 (i.e., $\delta'$ drops the curve $\delta$ to the straight line segment connection the points $(q/q_{\{2\}},\tau\cdot q/q_{\{2\}})$ and $(1,\delta)$).  This lower bounds revenue because considering $\pi_k$, for any price that it offers, for each realized value $v_{\{1\}}$ of agent 1, trade will occur with only possibly smaller probability under $\delta'$.

Now curves $\delta'$ and $\gamma$ both have constant slope in the input region $z\in\left[q/q_{\{2\}},1\right]$, i.e., they each have constant negative virtual values in this region.  And in particular, the constant virtual value of the $\delta'$ curve has (weakly) smaller magnitude than the constant virtual value of the $\gamma$ curve, as both curves go through the point $(q/q_{\{2\}},\tau\cdot q/q_{\{2\}})$, and they terminate respectively at $z=1$ at heights $\delta \geq \gamma$ by problem setup (the $\delta'$ curve does not drop as far from the peak).

We recall (from Myerson) that revenue can be calculated as the expectation over quantile of the dot product of the derivative of the revenue curve (which is virtual value) and allocation probability $y$, i.e.,
\begin{equation*}
    \text{Rev}(\texttt{ALG})=\mathbf{E}_q\left[y(q)\cdot \text{Rev}'(q)\right]
\end{equation*}
for $y$ the allocation rule as a function of quantile, from \texttt{ALG}.  However as we have already pointed out, $\left|\text{Rev}'_{\delta'}\right|\leq\left|\text{Rev}'_{\gamma}\right|$ in the analyzed region, additionally with the signs of the derivatives negative.  So we get a further reduction of our problem to showing the following argument: at each fixed $z\in\left[q/q_{\{2\}},1\right]$, allocation to agent 1 (with the allocation function induced by $\pi_k$) using $y_{\delta'}$ from the $\delta'$ curve and $v_{\delta'}$ mapping quantile $z$ to value, is smaller than allocation to agent 1 using $y_{\gamma}$ from the $\gamma$ curve and $v_{\gamma}$.  This is sufficient because- with virtual values as negative constants for each curve and the larger magnitude occurring with the $\gamma$ curve, the amortized analysis of revenue from virtual values in the equation will necessarily have smaller negative contribution for each quantile $z$ in this region using $\delta'$ compared to $\gamma$ (if this last statement holds).

We now relate an identity fact with respect to a {\em scaling factors} $\alpha \geq \alpha'$, regarding the CDF $\Pi_k$ (and PDF $\pi_k$ for completeness) of distributions which are scale-invariant in the lower bound of their support, like those we consider here.

\begin{align*}
\Pi_k(x)&=\Pi_{\alpha k}(\alpha x)\\
\Pi_k(x)&\geq\Pi_{\alpha k}(\alpha'x)\\
\pi_k(x)&=\alpha\cdot\pi_{\alpha k}(\alpha x)
\end{align*}

To invoke the second line here, for our fixed $z\in\left[q/q_{\{2\}},1\right]$, we let $k=\gamma$; and we let $\alpha = \delta/\gamma$; and we let $\alpha'=y_{\delta'(z)}/y_{\gamma(z)}$ which we can confirm is at most $\alpha$ by inspection.  Finally recognizing that the allocation rule is in fact the CDF of the pricing function in our analytical setting, the final required statement is proved such that pointwise for every fixed $z$, allocation is smaller using the $\delta'$ curve compared to the $\gamma$ curve.
\end{proof}

\noindent \textbf{Example scale-invariant pricing function: exponential}

We give the following example as illustrative support for the last two paragraphs of the proof.  The scale-invariant (in lower bound on support $k$) description of the exponential distribution is given by:
\begin{align*}
\text{cdf}: F_k(x) &= 1-e^{\frac{-1}{k}(x-k)}~\text{on}~ \left[k,\infty\right)\\
\text{pdf}: f_k(x) &= \frac{1}{k}\cdot e^{\frac{-1}{k}(x-k)}~\text{on}~ \left[k,\infty\right)
\end{align*}

If we use the exponential distribution $f_k$ as the scale-invariant pricing function $\pi_k$ with $k=v_{\{2\}}$, this induces the comparison
\begin{align*}
    F_{\delta}(z) &= 1-e^{\frac{-1}{\delta}(y_{\delta}(z)-\delta)} = 1-e\cdot e^{\frac{-1}{\delta}(y_{\delta}(z))}\\
    F_{\gamma}(z) &= 1-e^{\frac{-1}{\gamma}(y_{\gamma}(z)-\gamma)} = 1-e\cdot e^{\frac{-1}{\gamma}(y_{\gamma}(z))}
\end{align*}

Let the height of the curves $\delta'$ and and $\gamma$ at $z$ be denoted by $\mu_{\delta}\cdot\delta$ and $\mu_{\gamma}\cdot\gamma$ respectively, such that the heights factor out $\delta$ and $\gamma$ adding ``ratio" parameters $\mu_{\delta}$ and $\mu_{\gamma}$.  Then we have $y_{\delta}(z) = \mu_{\delta}\cdot \delta/z$ and $y_{\gamma}(z)=\mu_{\gamma}\cdot\gamma/z$.  Let $\mathbf{e}=e\cdot e^{1/z}$.  Substituting into the above we get
\begin{align*}
    F_{\delta}(z) &= 1-\mathbf{e}^{-\mu_{\delta}}\\
    F_{\gamma}(z) &= 1-\mathbf{e}^{-\mu_{\gamma}}
\end{align*}

Finally we compare the ratio parameters $\mu_{\delta}$ and $\mu{\delta}$.  Recall that $\mu{\delta}$ is the ratio of the height of the $\delta'$ curve at $z$, to $\delta$; and $\mu_{\gamma}$ analogous.  $\mu_{\delta}$ is clearly smaller in magnitude: its denominator $\delta$ is larger, and the increase from $\delta$ to its numerator is smaller than the increase from $\gamma$ to the numerator of $\mu_{\gamma}$, from the structure of the curves $\delta'$ and $\gamma$ (constant-slope lines through the same peak revenue point).

\noindent \textbf{Lemma Supporting the Truncation-step of the Triangle-Sufficiency proof}

\begin{lemma}
Given a fractional quantity
\begin{equation*}
    Q = \frac{\eta\cdot A' + B'}{\eta\cdot A'' + B''}
\end{equation*}
for $\eta, A', A'', B', B'' > 0$.  Let $A=A'/A''>0$ and $B=B'/B''>0$, then the following hold:
\begin{enumerate}
    \item if $A \geq B$, then $A\geq Q$;
    \item if $A \geq B$ (respectively equal to, less than), then $Q$ is increasing in $\eta$ (respectively constant, decreasing).
\end{enumerate}
\end{lemma}

\begin{proof}
Both statements are true by simple algebraic manipulation.  Note we re-arrange the assumption $A\geq B$ by $B'\leq (A'/A'')\cdot B''$.  For (1):
\begin{align*}
    Q = \frac{\eta\cdot A' + B'}{\eta\cdot A'' + B''} &\leq \frac{\eta\cdot A'+\frac{A'}{A''}B''}{\eta\cdot A'' + B''}\\
    &= \frac{\eta\cdot A'A''+A'B''}{A''(\eta\cdot A''+B'')}= \frac{A'(\eta\cdot A''+B'')}{A''(\eta \cdot A''+ B'')}=\frac{A'}{A''}
\intertext{For (2), first we take the derivative with respect to $\eta$ and work from there, with the last inequality equivalent to the assumption $A\geq B$:}
(\eta\cdot A''+ B'')^2\cdot \frac{\partial Q}{\partial \eta}&= (\eta\cdot A''+B'')\cdot A'-(\eta\cdot A'+B')\cdot A''\\
&= B''\cdot A' - B'\cdot A''\geq 0\qedhere
\end{align*}
\end{proof}

\begin{lemma}
Consider a negative-virtual value, regular, truncated revenue curve distribution, further lower-truncated and re-normalized at value $\zeta$.  I.e., it has truncation $\tau$ on the left side and achieves peak revenue at quantile $q$, and on the right side the revenue curve is concave (in quantile space) but ending at arbitrary point $(1,\zeta)$ for $\zeta\in\left[0,\tau\cdot q\right]$.  For this description, assume unbiased algorithms are parameterized by the lower truncation value $\zeta$.  For fixed $\zeta$, the revenue curve with smallest algorithm performance is the one with right hand side as a line segment connecting $(q,\tau\cdot q)$ to $(1,\zeta)$.
\end{lemma}
\begin{proof}
Having fixed $\zeta$, the prices offered by the unbiased algorithm are constant, independent of the rest of the revenue curve (which is implicitly unknown).  For any price offered, the line-segment revenue curve allocates with the smallest probability.  This ``dominating" property holds pointwise for all prices of a fixed mechanism, and is therefore sufficient.
\end{proof}

\begin{prop}
There exists a pricing distribution as input to an unbiased algorithm such that it is sufficient for the adversary to only ever consider triangle-revenue-curve distributions (including point masses as degenerate triangles).  In particular, the pricing function puts probability at most 1/2 on the second highest value $v_{\{2\}}=\zeta$.  Otherwise the pricing function uses the scale-free distribution which has cdf and ($\zeta$)-scaled-cdf:
\begin{align}
    \Pi(x) &= 1 - \frac{1}{x}~\text{{\em for}}~x\in[1,\infty)\\%^{1/2}}\\
    \Pi_{\zeta}(x)& =\Pi(\frac{x}{\zeta})= 1 - \left(\frac{\zeta}{x}\right)~\text{{\em for}}~x\in[\zeta,\infty)%^{1/2}
\end{align}
\end{prop}
\begin{proof}
First we note that the transformaton from scale-free $\Pi$ to $\Pi_{zeta}$ parameterized by scale $\zeta$ follows from the note after Definition~cref{def:scale} above.  The un-scaled density function is $\pi(x) = \frac{1}{x^2}$ for $x\in[1,\infty)$.%= \frac{1}{2}\cdot\frac{1}{(x+1)^{3/2}}$.

We adopt the technique of the previous proof and argue pointwise for every realized $v_{\{2\}} = \zeta$, which re-parameterizes the distribution of the high agent to be larger.  Draws of $q_{\{2\}}\leq q$ can be ignored because all considered revenue curves have the same structure in this range to the left of the peak, resulting in equal performance ex-post given these ``small" $q_{\{2\}}$.  The original revenue curve is normalized by dividing everywhere by $q_{\{2\}}$.  The truncation point is still $\tau$ but the peak revenue in quantile space is now $q/q_{\{2\}}$ for $q$ the original peak, and peak revenue is not $\tau\cdot q / q_{\{2\}}$.  That we can assume that the curve is truncated without loss was proved as part of the previous result.  Further, by the immediately preceding lemma, it is sufficient to only consider revenue curves with line segments connecting $(q,\tau\cdot q)$ to $(1,\zeta)$ on the right side of the peaks.

Our goal is to show for a fixed setting of $\zeta$, that with $\Pi,\Pi_{\zeta}$ as described, revenue of the algorithm is increasing with increasing $\zeta\in\left[0,\tau\cdot q/q_{\{2\}}\right]$.  We do this by analyzing the derivative of the revenue curve, with respect to $\zeta$.  This represents a change in both the ex-post realized value $v_{\{2\}}$ and correspondingly the scale-invariant pricing function.

%(Some quick notes before giving the analysis.  The sub-calculations for $v_{\zeta}(z)$ and $v_{\zeta}(z)/\zeta$ and its derivative for chain-rule are given at the bottom.  Also, recall we analyze the revenue of pricing function $\Pi_{\zeta}$ which is only part of the total pricing function.  It is less than half the weight, with at least half the weight of the pricing function setting a price of $v_{\{\2\}}$.)

\begin{align}
    \text{Rev}_{\zeta} &= \mathbf{E}_q\left[R'(q)\cdot \Pi_{\zeta}(q)\right]= \int_0^1 R'(q)\cdot \Pi_{\zeta}(v_{\zeta}(z))dz\\
    &= \left(\frac{\tau q}{q_{\{2\}}}\right)\cdot \Pi_{\zeta}(\tau)+\left(\frac{\zeta-\tau q/q_{\{2\}}}{1-q/q_{\{2\}}} \right)\cdot\int_{q/q_{\{2\}}}^1\Pi_{\zeta}(v_{\zeta}(z))dz\\
    &= \left(\frac{\tau q}{q_{\{2\}}}\right)\cdot \Pi(\frac{\tau}{\zeta})-\left(\frac{\tau q/q_{\{2\}}-\zeta}{1-q/q_{\{2\}}} \right)\cdot\int_{q/q_{\{2\}}}^1\Pi(\frac{v_{\zeta}(z)}{\zeta})dz
\intertext{(as mentioned, the calculation of the derivative of $v_{\zeta}(z)/\zeta$ is given at the end of the proof)}
\label{eqn:revderiv}
    \frac{\partial \text{Rev}_\zeta}{\partial \zeta} &= \left(\frac{\tau q}{q_{\{2\}}} \right)\cdot \pi(\frac{\tau}{\zeta})\cdot\left(\frac{-\tau}{\zeta^2}\right)+\left(\frac{1}{1-q/q_{\{2\}}} \right)\cdot\int_{q/q_{\{2\}}}^1\Pi(\frac{v_{\zeta}(z)}{\zeta})dz\\
    &-\left(\frac{\tau q/q_{\{2\}}-\zeta}{q-q_{\{2\}}} \right)\cdot\int_{q/q_{\{2\}}}^1\pi(\frac{v_{\zeta}(z)}{\zeta})\cdot\left(\frac{-1}{\zeta^2}\right)\cdot\left(\frac{\tau q / q_{\{2\}}}{1-q/q_{\{2\}}}\right)\cdot\left(\frac{1-z}{z} \right)dz\\
\intertext{(we drop the last two additive terms which are positive; and substitute in the definition of our existential $\pi$ function; note that we should not think of $\pi$ here as being used as a density function; rather, it is the result of the calculus within a chain-rule operation, we use it directly as the resulting function evaluated on its input, it does not have an economic interpretation as density here (in $x$) as it is the derivative with respect to scale $\zeta$)}
\label{eqn:partrevpartzeta}
    &\geq \left(\frac{\tau q}{q_{\{2\}}} \right)\cdot \left[ \frac{1}{\left(\tau/\zeta\right)^2} \right]\cdot\left(\frac{-\tau}{\zeta^2}\right)=-1\cdot \left(\frac{q}{q_{\{2\}}} \right)\geq -1%%+\left(\frac{1}{1-q/q_{\{2\}}} \right)\cdot\int_{q/q_{\{2\}}}^1\Pi(\frac{v_{\zeta}(z)}{\zeta}-1)dz\\
    %&+\left(\frac{\tau q/q_{\{2\}}-\zeta}{q-q_{\{2\}}} \right)\cdot\int_{q/q_{\{2\}}}^1\pi(\frac{v_{\zeta}(z)}{\zeta}-1)\cdot\left(\frac{1}{\zeta^2}\right)\cdot\left(\frac{\tau q / q_{\{2\}}}{1-q/q_{\{2\}}}\right)\cdot\left(\frac{1-z}{z} \right)dz\\
\end{align}
\noindent which is finally sufficient, because the analysis here is for $\Pi_{\zeta}$ which is used at most half of the time by the pricing function of the unbiased algorithm.  At least half of the time, the pricing function runs the second-price auction using a fixed price of $v_{\{2\}}$.  The contribution to the (un-normalized to total weight 1) partial derivative $\partial \text{Rev}_{\zeta}/\partial \zeta$ of the point mass is simply `$+1$' from its (conditional) revenue of $\zeta$.  Having more than half the weight and combining with line~\eqref{eqn:partrevpartzeta} shows the total derivative is non-negative as desired.

In conclusion.  Given our choice of $\Pi$, algorithm revenue is minimized pointwise per $v_{\{2\}}$ by the ex-post revenue curve with structure to the right of the peak as a straight line segment connecting revenue curve points $(q/q_{\{2\}},\tau q/q_{\{2\}})$ to $(1,v_{\{2\}}$).  This property can only be achieved by triangle revenue curve distributions, which as a consequence of our analysis in this proof dominate all other distributions (in terms of minimizing algorithm revenue).

The remainder of the proof just gives the deferred calculations for the chain-rule term.  The starting definition follows from the revenue curve graph:

\begin{align*}
    v_{\zeta}(z)&= \frac{\zeta+\left(\frac{(1-z)}{1-q/q_{\{2\}}} \right)\cdot \left(\frac{\tau q}{q_{\{2\}}}-\zeta\right)}{z}\\
    &= \frac{\zeta+\left(\frac{(1-z)}{q_{\{2\}}-q} \right)\cdot \left(\tau q-\zeta\cdot q_{\{2\}}\right)}{z}=\frac{\zeta(q_{\{2\}}-q)+(1-z)\cdot \left(\tau q-\zeta\cdot q_{\{2\}}\right)}{z(q_{\{2\}}-q)}\\
    &= \frac{\zeta q_{\{2\}}-\zeta q + \tau q -\zeta q_{\{2\}}-z\tau\zeta q +z\zeta q_{\{2\}}}{z(q_{\{2\}}-q)}=\frac{\zeta(zq_{\{2\}}-q)+\tau q(1-z)}{z(q_{\{2\}}-q)}\\
    \frac{v_{\zeta}(z)}{\zeta}&= \frac{zq_{\{2\}}-q}{z(q_{\{2\}}-q}+\frac{\tau q (1-z)}{z(q_{\{2\}}-q)\zeta}\\
    \frac{\partial\left(v_{\zeta}(z)/\zeta \right)}{\partial \zeta} &= \left(\frac{-1}{\zeta^2}\right)\cdot\left(\frac{\tau q (1-z)}{z(q_{\{2\}}-q)} \right) = \left( \frac{-1}{\zeta^2}\right)\cdot\left(\frac{\tau q / q_{\{2\}}}{1-q/q_{\{2\}}}\right)\cdot\left(\frac{1-z}{z} \right)\qedhere
\end{align*}
\end{proof}

\noindent \textbf{Further analysis}

%The previous statement further holds using the following distribution as the scale-invariant pricing function input.  

The previous statement does not hold everywhere for the following.  It does not hold if we consider inverse-exponential function, truncate it below at $x=1$, and re-normalize its density by dividing through by $(1-e^{-1})$.  However if we change the minimum setting of probability on the point mass $\beta\approx 0.6127$, we have the analogous similar result.  Also it does not hold when using the exponential function, but holds for $\beta \approx 0.5954$.

We work from line~\eqref{eqn:revderiv} in the previous proof, again dropping two terms and this time replacing $\pi(\frac{\tau}{\zeta})$ with first the inverse-exponential distribution version of the scale invariant pdf, and below the exponential distribution.  First the function is $\pi(x) = \frac{e}{e-1}\cdot\frac{1}{x^2}\cdot e^{-1/x}$ on $[1,\infty)$.  We get
\begin{align}
    \frac{\partial \text{Rev}_\zeta}{\partial \zeta} &= \left(\frac{\tau q}{q_{\{2\}}} \right)\cdot \pi(\frac{\tau}{\zeta})\cdot\left(\frac{-\tau}{\zeta^2}\right)+\left(\frac{1}{1-q/q_{\{2\}}} \right)\cdot\int_{q/q_{\{2\}}}^1\Pi(\frac{v_{\zeta}(z)}{\zeta})dz\\
    &-\left(\frac{\tau q/q_{\{2\}}-\zeta}{q-q_{\{2\}}} \right)\cdot\int_{q/q_{\{2\}}}^1\pi(\frac{v_{\zeta}(z)}{\zeta})\cdot\left(\frac{-1}{\zeta^2}\right)\cdot\left(\frac{\tau q / q_{\{2\}}}{1-q/q_{\{2\}}}\right)\cdot\left(\frac{1-z}{z} \right)dz\\
    &\geq \left(\frac{\tau q}{q_{\{2\}}} \right)\cdot \left[\frac{e}{e-1}\cdot\frac{1}{(\tau/\zeta)^2}\cdot e^{-\zeta/\tau}\right]\cdot\left(\frac{-\tau}{\zeta^2}\right)=\left(\frac{-q}{q_{\{2\}}} \right)\cdot \left[\frac{e}{e-1}\cdot e^{-\zeta/\tau}\right]
\end{align}
We can change the probability on the point mass $\beta$ as follows, and then the anologous result goes through.

\begin{align*}
    \beta + (1-\beta)\cdot \left[-1\cdot(e/(e-1))\right] &\geq 0\\
    \beta & \geq (1-\beta)\cdot \left[(e/(e-1))\right]\\
    \beta(1+e/(e-1))&\geq e/(e-1)\\
    \beta &\geq \frac{e/(e-1)}{1+e/(e-1)}=e/(2e-1)\approx 0.6127
\end{align*}

\noindent Next the function is $\pi(x)=e^{-(x-1)}$ on $[1,\infty)$.\footnote{Note that because exponential distributions are normally defined on a range $[0,\infty)$, and this is independent of scale, we must replace $x$ with $(x-1)$ within the normal pdf definition to have the pdf range be $[1,\infty)$ for our scale-invariance.}  We get

\begin{align}
    \frac{\partial \text{Rev}_\zeta}{\partial \zeta} &= \left(\frac{\tau q}{q_{\{2\}}} \right)\cdot \pi(\frac{\tau}{\zeta})\cdot\left(\frac{-\tau}{\zeta^2}\right)+\left(\frac{1}{1-q/q_{\{2\}}} \right)\cdot\int_{q/q_{\{2\}}}^1\Pi(\frac{v_{\zeta}(z)}{\zeta})dz\\
    &-\left(\frac{\tau q/q_{\{2\}}-\zeta}{q-q_{\{2\}}} \right)\cdot\int_{q/q_{\{2\}}}^1\pi(\frac{v_{\zeta}(z)}{\zeta})\cdot\left(\frac{-1}{\zeta^2}\right)\cdot\left(\frac{\tau q / q_{\{2\}}}{1-q/q_{\{2\}}}\right)\cdot\left(\frac{1-z}{z} \right)dz\\
    &\geq \left(\frac{\tau q}{q_{\{2\}}} \right)\cdot \left[ e^{-(\tau/\zeta-1)}\right]\cdot\left(\frac{-\tau}{\zeta^2}\right)= \left(\frac{-q}{q_{\{2\}}}\right)\cdot e \cdot \left[\frac{\tau^2}{\zeta^2}\cdot e^{-(\tau/\zeta-1)}\right]
\end{align}
\noindent We analyze the last term as follows.  Consider function $h(x)=x^2\cdot e^{-(x-1)}$ on $[0,\infty)$.  The relevance of this is that we see $h(\tau/\zeta) = (\tau/\zeta)^2\cdot e^{-(\tau/\zeta-1)}$ in the brackets.  The function $h$ is not smaller than 1 for all positive inputs, but $\tau/\zeta$ can evaluate to the full range of positive reals.  To see this, we check its derivative as $h'(x) = (2x-x^2)\cdot e^{-(x-1)}$, which is positive for $x\in[0,2]$ and negative everywhere afterwards.  Therefore the function $h$ peaks at input $x=2$.  Evaluating $h(2) = 4\cdot e^{-1}$, so it is not smaller than 1 everywhere.  However, if we increase the probability on the point mass on $v_{\{2\}}$ from its current setting of 0.5, the exponential distribution could be used; the probability of the point mass $\beta$ versus the probability of $\Pi$ instead needs to be lower bounded to satisfy
\begin{align*}
    \beta + (1-\beta)\cdot \left[-1\cdot(4\cdot e^{-1})\right] &\geq 0\\
    \beta & \geq (1-\beta)\cdot \left[(4\cdot e^{-1})\right]\\
    \beta(1+4/e)&\geq 4/e\\
    \beta &\geq \frac{4/e}{1+4/e}\approx 0.5954
\end{align*}

\noindent The following lemma does not have a specific purpose yet, but I want to get it recorded.  It translates an integral over $\Pi$ into a quantity using $\pi$.  However I think it might be too ``lossy" of a lower bound on a positive term.

\begin{lemma}
For an unbiased algorithm, in the analysis of the derivative of Revenue with respect to $\zeta=v_{\{2\}}$, if the density of the random pricing function $\Pi_{\zeta}$ is non-increasing (in value), then the second term is lower bounded as 
\begin{equation}
    \left(\frac{1}{1-q/q_{\{2\}}} \right)\cdot\int_{q/q_{\{2\}}}^1\Pi(\frac{v_{\zeta}(z)}{\zeta})dz\geq 2\left(1-\frac{q}{q_{\{2\}}}\right)\cdot \pi_{\zeta}(\tau)
\end{equation}
\end{lemma}
\begin{proof}
We give the calculation with explanation of steps inline:
\begin{align*}
    \left(\frac{1}{1-q/q_{\{2\}}} \right)\cdot\int_{q/q_{\{2\}}}^1\Pi(\frac{v_{\zeta}(z)}{\zeta})dz &= \left(\frac{1}{1-q/q_{\{2\}}} \right)\cdot\int_{q/q_{\{2\}}}^1\left[\Pi_{\zeta}(z)\right]dz\\
\intertext{(the right-hand side above is the average height of the pricing function cdf in quantile space in the range $[q/q_{\{2\}},1]$, which is a weakly decreasing and weakly concave curve by the assumption that pricing density is non-decreasing in value)}
    &= \left(\frac{1}{1-q/q_{\{2\}}} \right)\cdot\int_{q/q_{\{2\}}}^1\left[\int_1^z \pi_{\zeta}(y) dy\right] dz\\
    &\geq \left(\frac{1}{1-q/q_{\{2\}}} \right)\cdot\int_{q/q_{\{2\}}}^1\left[\int_1^z \left(\frac{\Pi_{\zeta}(q/q_{\{2\}})}{1-q/q_{\{2\}}}\right)dy\right] dz
\intertext{(for the inner integral, we can lower bound the height at each $z$ by replacing cumulative density with the average, by concavity; this quantity is now the ``average" height of the lower bound straight line pricing function connecting $(q/q_{\{2\}},\Pi_{\zeta}(\tau)$ and $(1,0)$, whose average is trivially half of $\Pi_{\zeta}(\tau)$)}
    &= \frac{1}{2}\cdot \Pi_{\zeta}(\tau) \geq \left(1-\frac{q}{q_{\{2\}}}\right)\cdot \pi_{\zeta}(\tau)
\end{align*}
\noindent with the last inequality following because with $\Pi_{\zeta}$ concave and decreasing and ending at a ``height" of 0 at $(1,0)$, the smallest (magnitude) derivative occurs at the smallest input $q/q_{\{2\}}$ with magnitude $\Pi_{\zeta}(\tau)$ and the ``height gain" applying this slope over a range of $1-q/q_{\{2\}}$ can not be larger than the height of the cumulative.
\end{proof}

\subsection{Analysis of pricing functions against Uniform distributions}

This section is an analysis of the original benchmark optimal resolution program, for which there is at least some small reason to believe that downward-closed Uniform distributions could be the critical blend on one side.  This follows from noting that one side is very likely to be upward closed equal revenue distributions, and the past observed importance of the weights having "ratio" between them proportional to $1/z$, which is the weight used for the technique to find dual blends of using the $1/z$-inverse distribution given a starting scale-invariant CDF.
