# Supplementary material for: Benchmark Design and Prior-independent Optimization
Source: arXiv:2001.10157 source file (2020-09-08)
Supplement: Supplementary file 2 [file yingkai_notes.tex]

\section{Yingkai Notes}
The algorithm chooses a point mass $\mass$ on value 1 
and a density function $\density(\ratio)$ 
supported on $[1, \infty)$
such that 
\begin{align*}
\mass + \int_1^\infty \density(\ratio) d\val = 1.
\end{align*}

The adversary is constrained to choose triangle distributions 
with maximum revenue equal to~1. 
For triangle distributions, 
given the cutoff quantile $\cutoffq$, 
the triangle distribution has valuation function 
\begin{equation*}
\valf(\quant) = 
\begin{cases}
\frac{1-\quant}{\quant(1-\cutoffq)} & \quant \geq \cutoffq, \\
\frac{1}{\cutoffq} & o/w.
\end{cases}
\end{equation*}
The optimal revenue given the cutoff quantile $\cutoffq$ is
$$\OPT(\quant) = 2-\cutoffq.$$ 

First note that the quantile 
corresponding to the price of $\quant$ 
scaled up by a ratio of $\ratio \geq 1$ is 
$$\ScaledQuant(\quant, \ratio) = \frac{\quant}{\ratio - \quant\ratio + \quant}.$$

The revenue of pricing function with $\mass, \density$ 
given distribution with quantile $\cutoffq$ is 
\begin{eqnarray*}
\Rev{\mass,\density; \cutoffq}
&=& \alpha \cutoffq^2 
\cdot \valf(\cutoffq) 
+
2\alpha 
\int_{\cutoffq}^{1}
\valf(\quant) \quant
\,d\quant
\\ 
&&+ 
2\int_1^\infty \density(\ratio) \cdot \ratio 
\int_{\ScaledQuant(\cutoffq, \sfrac{1}{\ratio})}^{1}
\valf(\quant) 
\ScaledQuant(\quant, \ratio)
\,d\quant \,d\ratio\\
&=& 
\alpha \cutoffq 
+ 
2\alpha 
\int_{\cutoffq}^{1}
\frac{1-\quant}{1-\cutoffq}
\,d\quant
\\
&&+ 
2\int_1^\infty \density(\ratio) \cdot \ratio 
\int_{\ScaledQuant(\cutoffq, \sfrac{1}{\ratio})}^{1}
\frac{1-\quant}{1-\cutoffq} \cdot 
\frac{1}{\ratio - \quant\ratio + \quant}
\,d\quant \,d\ratio\\
&=& \alpha \cutoffq 
+ \alpha (1-\cutoffq)
\\
&&+ 
2\int_1^\infty \density(\ratio) 
\cdot \frac{\ratio}{(1-\cutoffq)(\ratio-1)}
\int_{\ScaledQuant(\cutoffq, \sfrac{1}{\ratio})}^{1}
\left(1- 
\frac{1}{\ratio - \quant\ratio + \quant}
\right)
\,d\quant \,d\ratio\\
&=& \alpha \cutoffq 
+ \alpha (1-\cutoffq)
\\
&&+ 
\frac{2}{1-\cutoffq}\int_1^\infty \density(\ratio) \cdot 
\frac{\ratio}{(1-\cutoffq)(\ratio-1)} 
\left(
\frac{1-\cutoffq}{1-\cutoffq+\cutoffq\ratio}
+
\frac{\ln \left(
\frac{\ratio}{1-\cutoffq+\cutoffq\ratio}
\right)}{1-\ratio}
\right) \,d\ratio
\end{eqnarray*}

% \begin{eqnarray*}
% \Rev{\mass,\density; \cutoffq}
% &=& \alpha \\
% &&+ 
% \int_1^\infty \density(\ratio) \cdot \ratio 
% \left[\cutoffq \cdot 
% \int_{\ScaledQuant(\cutoffq, \ratio)}^1 
% \valfunc(\quant') d\quant'
% +
% \int_{\cutoffq}^1 \int_{\ScaledQuant(\quant, \ratio)}^1 
% \valfunc(\quant') d\quant' \,d\quant
% +
% \ScaledQuant(1, \frac{1}{\ratio})
% \int_{\cutoffq}^{\ScaledQuant(1, \ratio)}
% \valfunc(\quant) \,d\quant
% \right]
% \end{eqnarray*}

\subsection{Focusing on lookahead mechanisms}
Let $\regular$ be the set of regular distributions, 
and $\tri$ be the set of triangle distributions. 
Let $\scalei$ be the set of scale invariant mechanisms and $\sfl$ be the set of scale invariant and look ahead mechanisms. 

\begin{eqnarray*}
&&\max_{\mecha \in \Delta(\sfl)}
\min_{\dist \in \regular}\Rev{\mecha, \dist}
= \max_{\mecha \in \Delta(\sfl)}
\min_{\dist \in \tri}\Rev{\mecha, \dist} \\
&=& \min_{\dist \in \Delta(\tri)}
\max_{\mecha \in \sfl}
\Rev{\mecha, \dist}
= \min_{\dist \in \Delta(\tri)}
\max_{\mecha \in \scalei}
\Rev{\mecha, \dist} \\
&\geq& \min_{\dist \in \Delta(\regular)}
\max_{\mecha \in \scalei}
\Rev{\mecha, \dist}
= \max_{\mecha \in \Delta(\scalei)}
\min_{\dist \in \regular}
\Rev{\mecha, \dist}
\end{eqnarray*}

The first inequality holds by \Cref{...}. 
The second and the last equality holds by min-max theorem. 
The third equality holds because for any mechanism $\mecha$, 
there exists a lookahead mechanism $\mecha'$ 
such that the revenue of $\mecha'$ is weaker higher for all 
triangle distributions. 
The inequality holds since the distribution is chosen from a larger set. 

Since we know that 
$\max_{\mecha \in \Delta(\scalei)}
\min_{\dist \in \regular}
\Rev{\mecha, \dist} 
\geq \max_{\mecha \in \Delta(\sfl)}
\min_{\dist \in \regular}\Rev{\mecha, \dist}$. 
Combining the two inequalities, 
we have 
$$\max_{\mecha \in \Delta(\scalei)}
\min_{\dist \in \regular}
\Rev{\mecha, \dist} 
= \max_{\mecha \in \Delta(\sfl)}
\min_{\dist \in \regular}\Rev{\mecha, \dist}.$$
\newpage
